# Supplementary material for: Not all Views are Created Equal: Analyzing Viewpoint Instabilities in Vision Foundation Models
Source: arXiv:2412.19920 source file (2024-12-27)
Supplement: Supplementary file 1 [file X_suppl.tex]

\clearpage
\setcounter{page}{1}
\maketitlesupplementary

This supplementary material includes additional experimental results that complement the findings presented in the main paper. Specifically, we provide:

\begin{itemize}
\item Additional results on label overlap across nine featurizers for stable, accidental, and OOD viewpoints, evaluated using pairwise Intersection over Union (IoU) heatmaps.
    \item Cluster samples from accidental and OOD viewpoints for seven additional featurizers not included in the main paper. These examples highlight consistent trends and instabilities in viewpoint classification.
    \item Expanded qualitative examples of Visual Question Answering (VQA) using LLaVA-1.5, which demonstrate the model's strengths and limitations across stable, accidental, and OOD viewpoints.
    \item Additional single-view monocular 3D reconstruction results. These examples further illustrate the impact of viewpoint instability on reconstruction accuracy, emphasizing the challenges posed by accidental and OOD viewpoints.
\end{itemize}

\section{Featurizer Agreement on Viewpoint Labels}

We present additional results on the level of agreement, measured using Intersection over Union (IoU), across the nine featurizers in identifying stable, accidental, and OOD viewpoints. Specifically, we provide IoU heatmaps for each category across all nine featurizers (see Fig.~\ref{fig:merged_figure}). 
The results indicate consistent trends: all featurizers exhibit strong agreement on stable viewpoints (IoU scores ranging from 0.98 to 1.00), moderate agreement on accidental viewpoints (IoU scores between 0.34 and 0.83), and very little agreement on OOD viewpoints (IoU scores ranging from 0.02 to 0.28). 
For accidental viewpoints, the moderate agreement suggests that these challenging viewpoints are generally identified similarly across featurizers, demonstrating some commonality in how models handle such instances. In contrast, the lack of agreement for OOD viewpoints, with many pairs of featurizers showing no overlap (IoU scores under 0.1), highlights the model-specific nature of viewpoint instability. This underscores the challenge of constructing datasets or methods that generalize viewpoint invariance across models. The results suggest that while accidental viewpoint invariance may benefit from shared strategies across models, OOD viewpoint invariance likely needs to be tailored to specific featurizers rather than assuming a universal approach.

\begin{figure*}
    \centering
    % First row: Fig 1 and Fig 2
    \begin{subfigure}{0.48\textwidth}
        \centering
        \includegraphics[width=\textwidth, trim=5cm 2cm 0 0, clip]{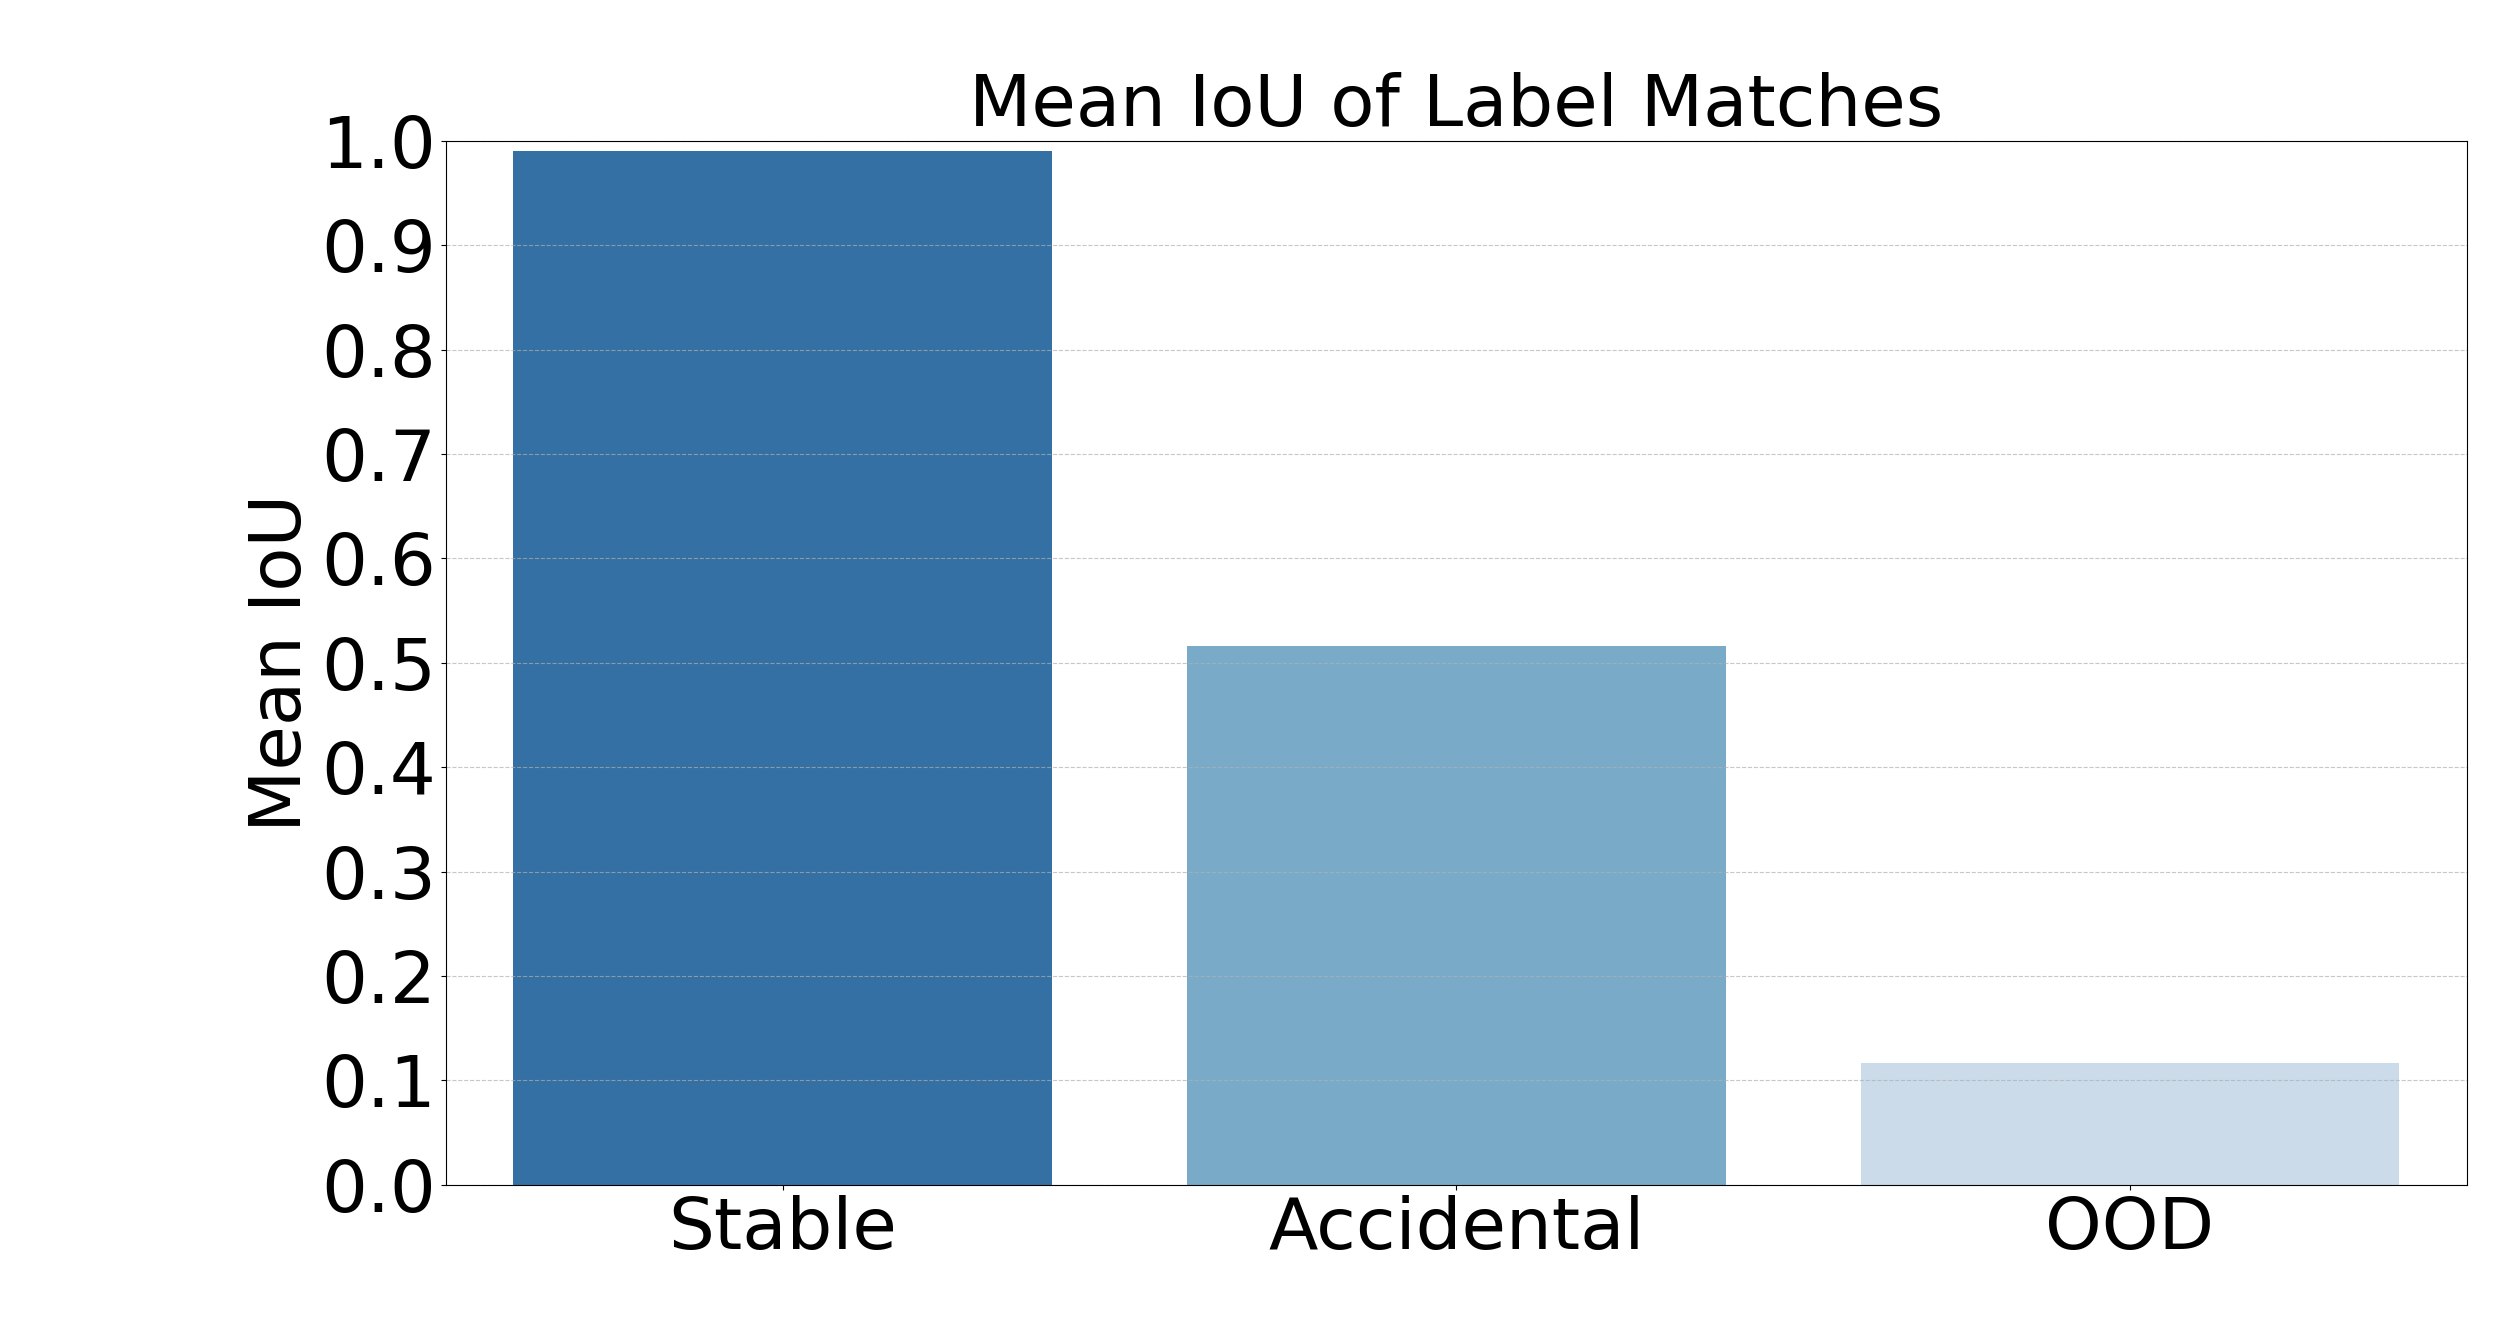}
        % \caption{Caption0.}
        \label{fig:subfig_mean}
    \end{subfigure}
    \hfill
    \begin{subfigure}{0.48\textwidth}
        \centering
        \includegraphics[width=\textwidth, trim=7cm 2cm 0 0, clip]{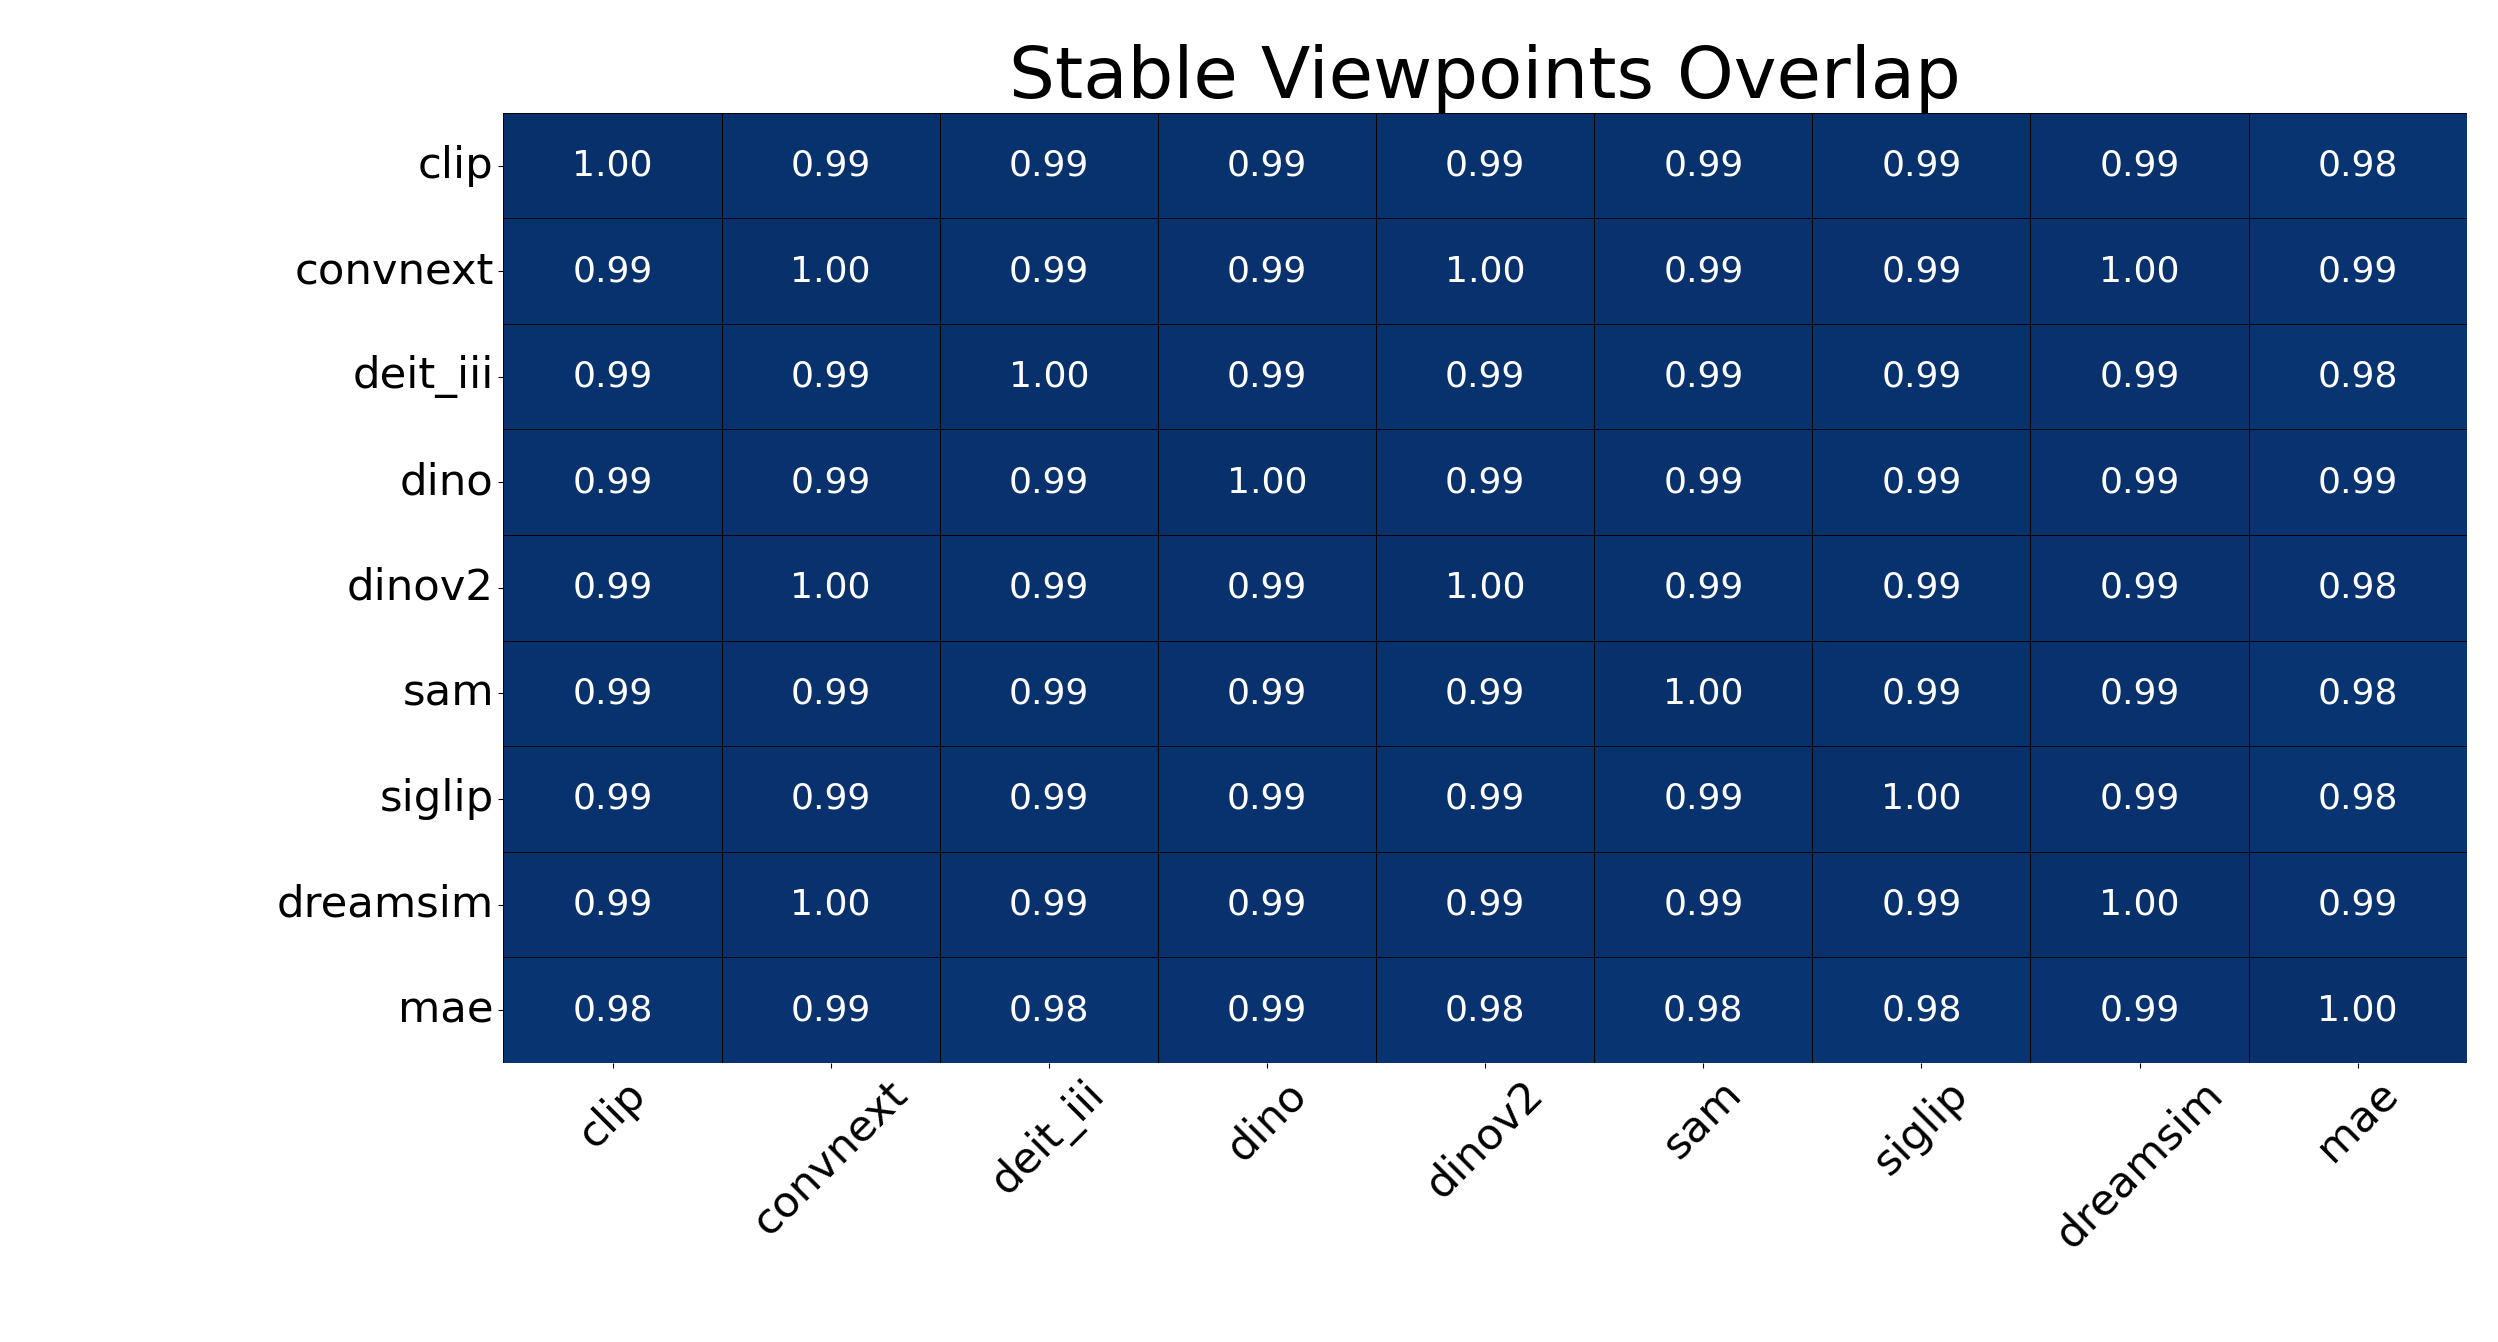}
        % \caption{Caption1 (Stable).}
        \label{fig:subfig_stable}
    \end{subfigure}
    \vspace{0.5cm}
    % Second row: Fig 3 and Fig 4
    \begin{subfigure}{0.48\textwidth}
        \centering
        \includegraphics[width=\textwidth, trim=7cm 2cm 0 0, clip]{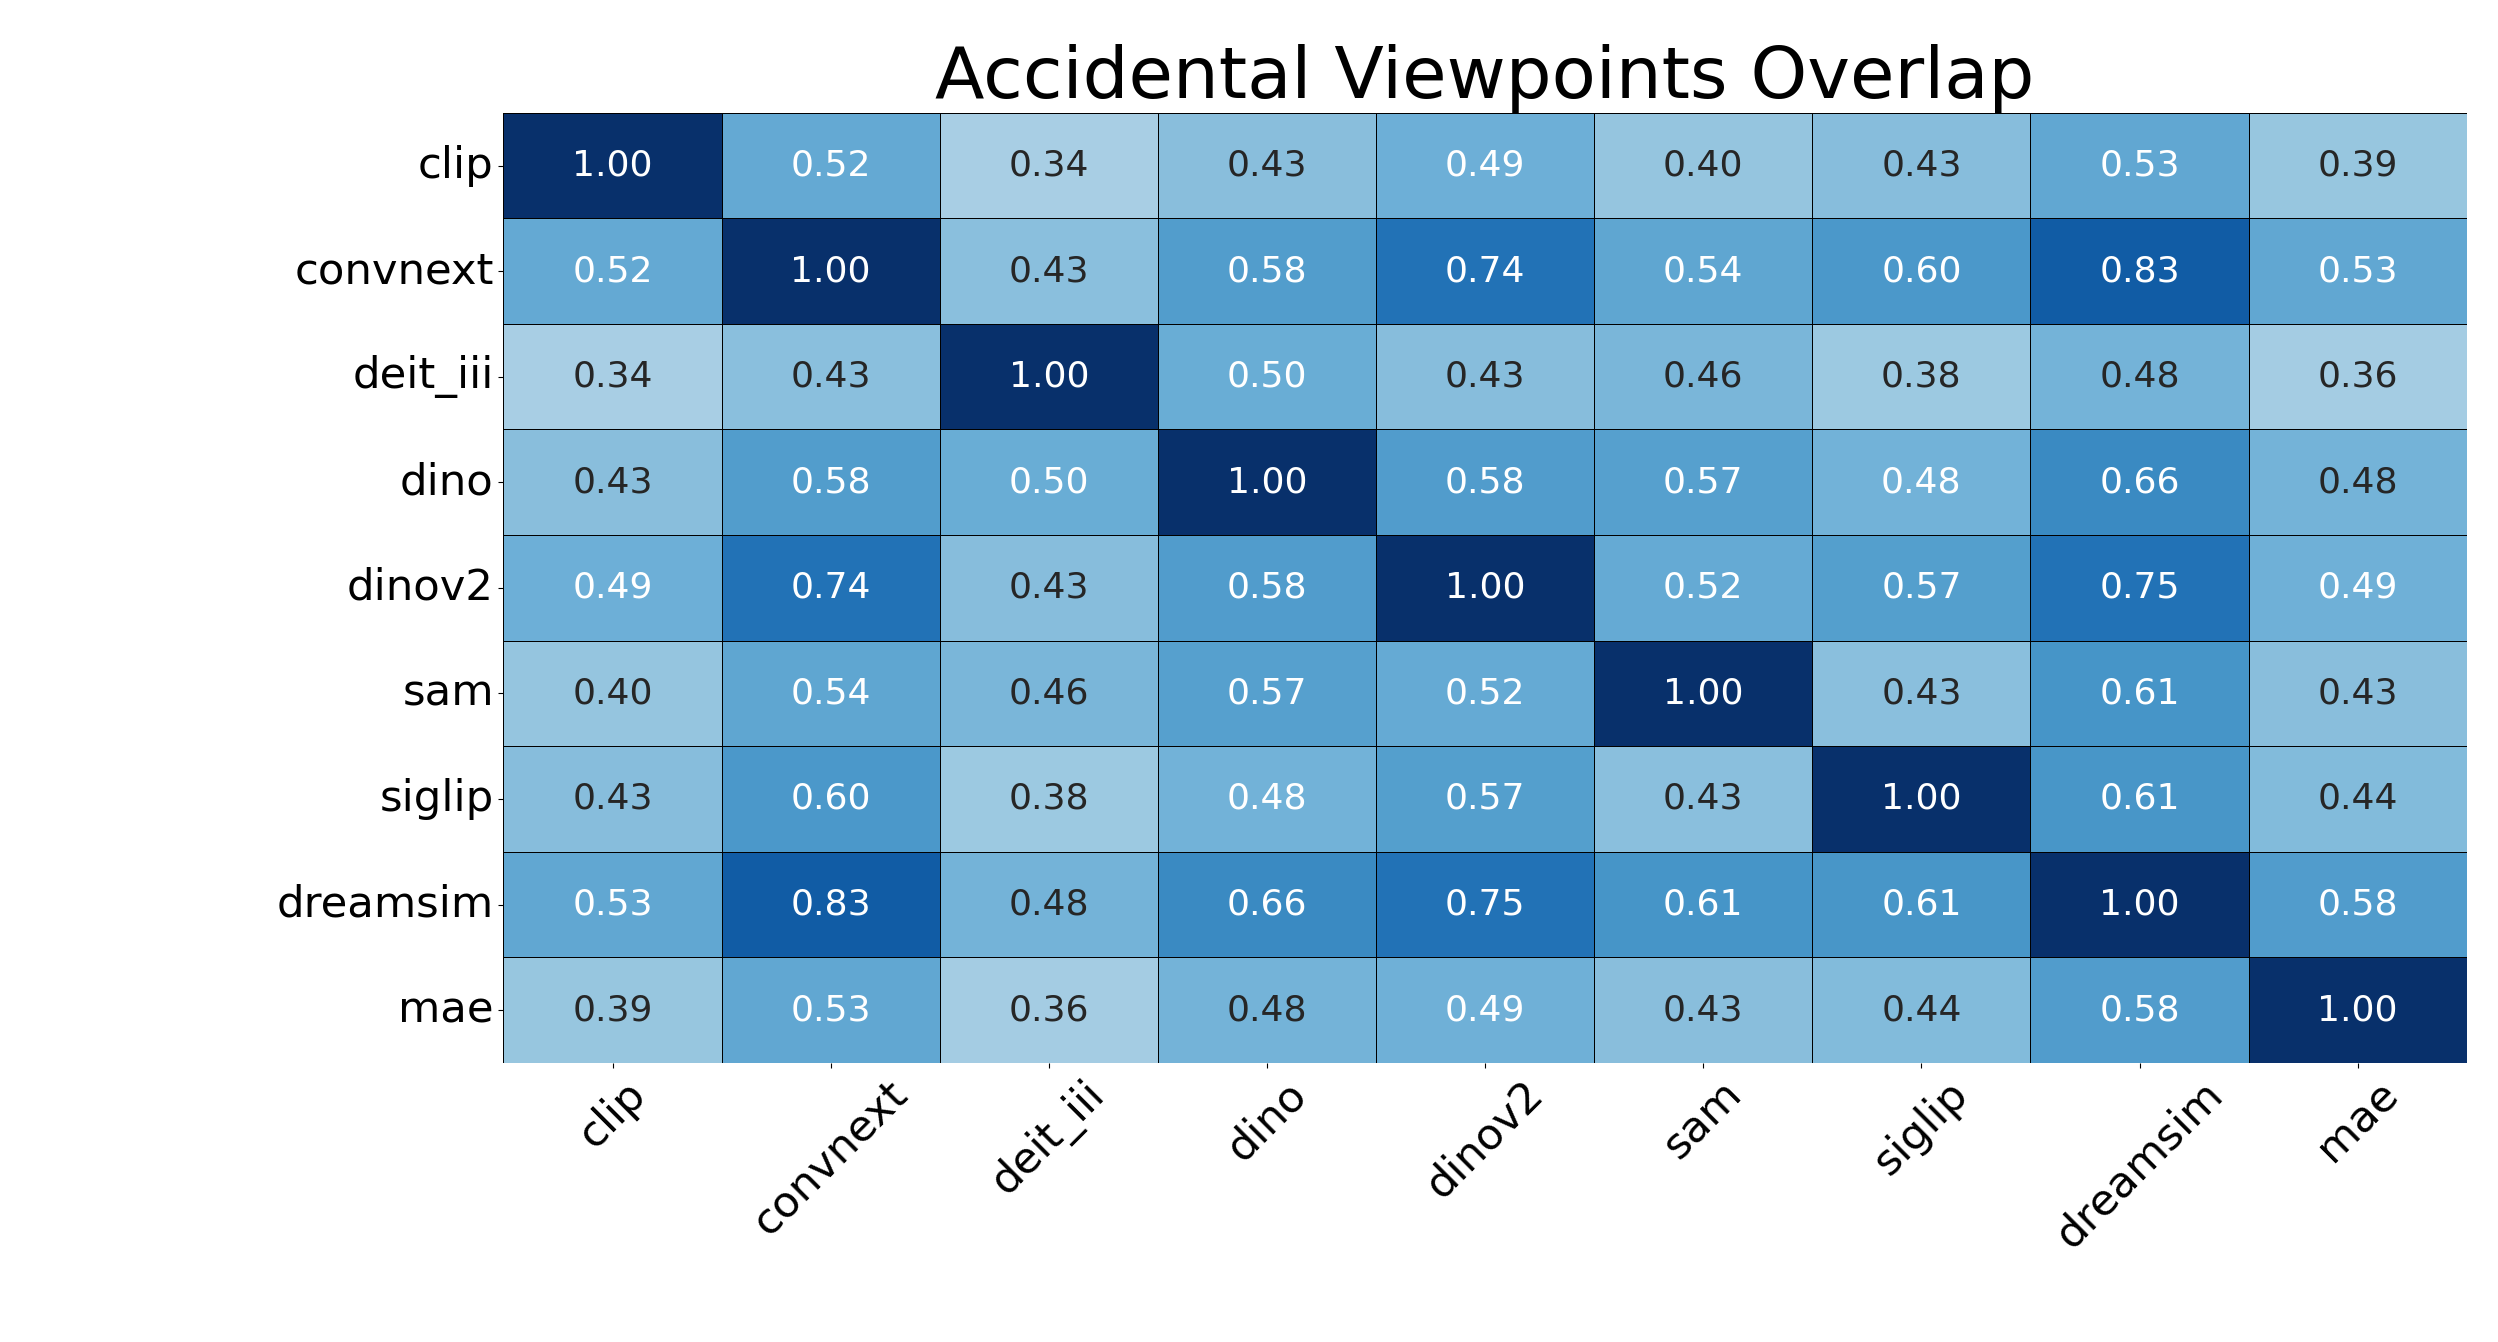}
        % \caption{Caption1 (Accidental).}
        \label{fig:subfig_accidental}
    \end{subfigure}
    \hfill
    \begin{subfigure}{0.48\textwidth}
        \centering
        \includegraphics[width=\textwidth, trim=7cm 2cm 0 0, clip]{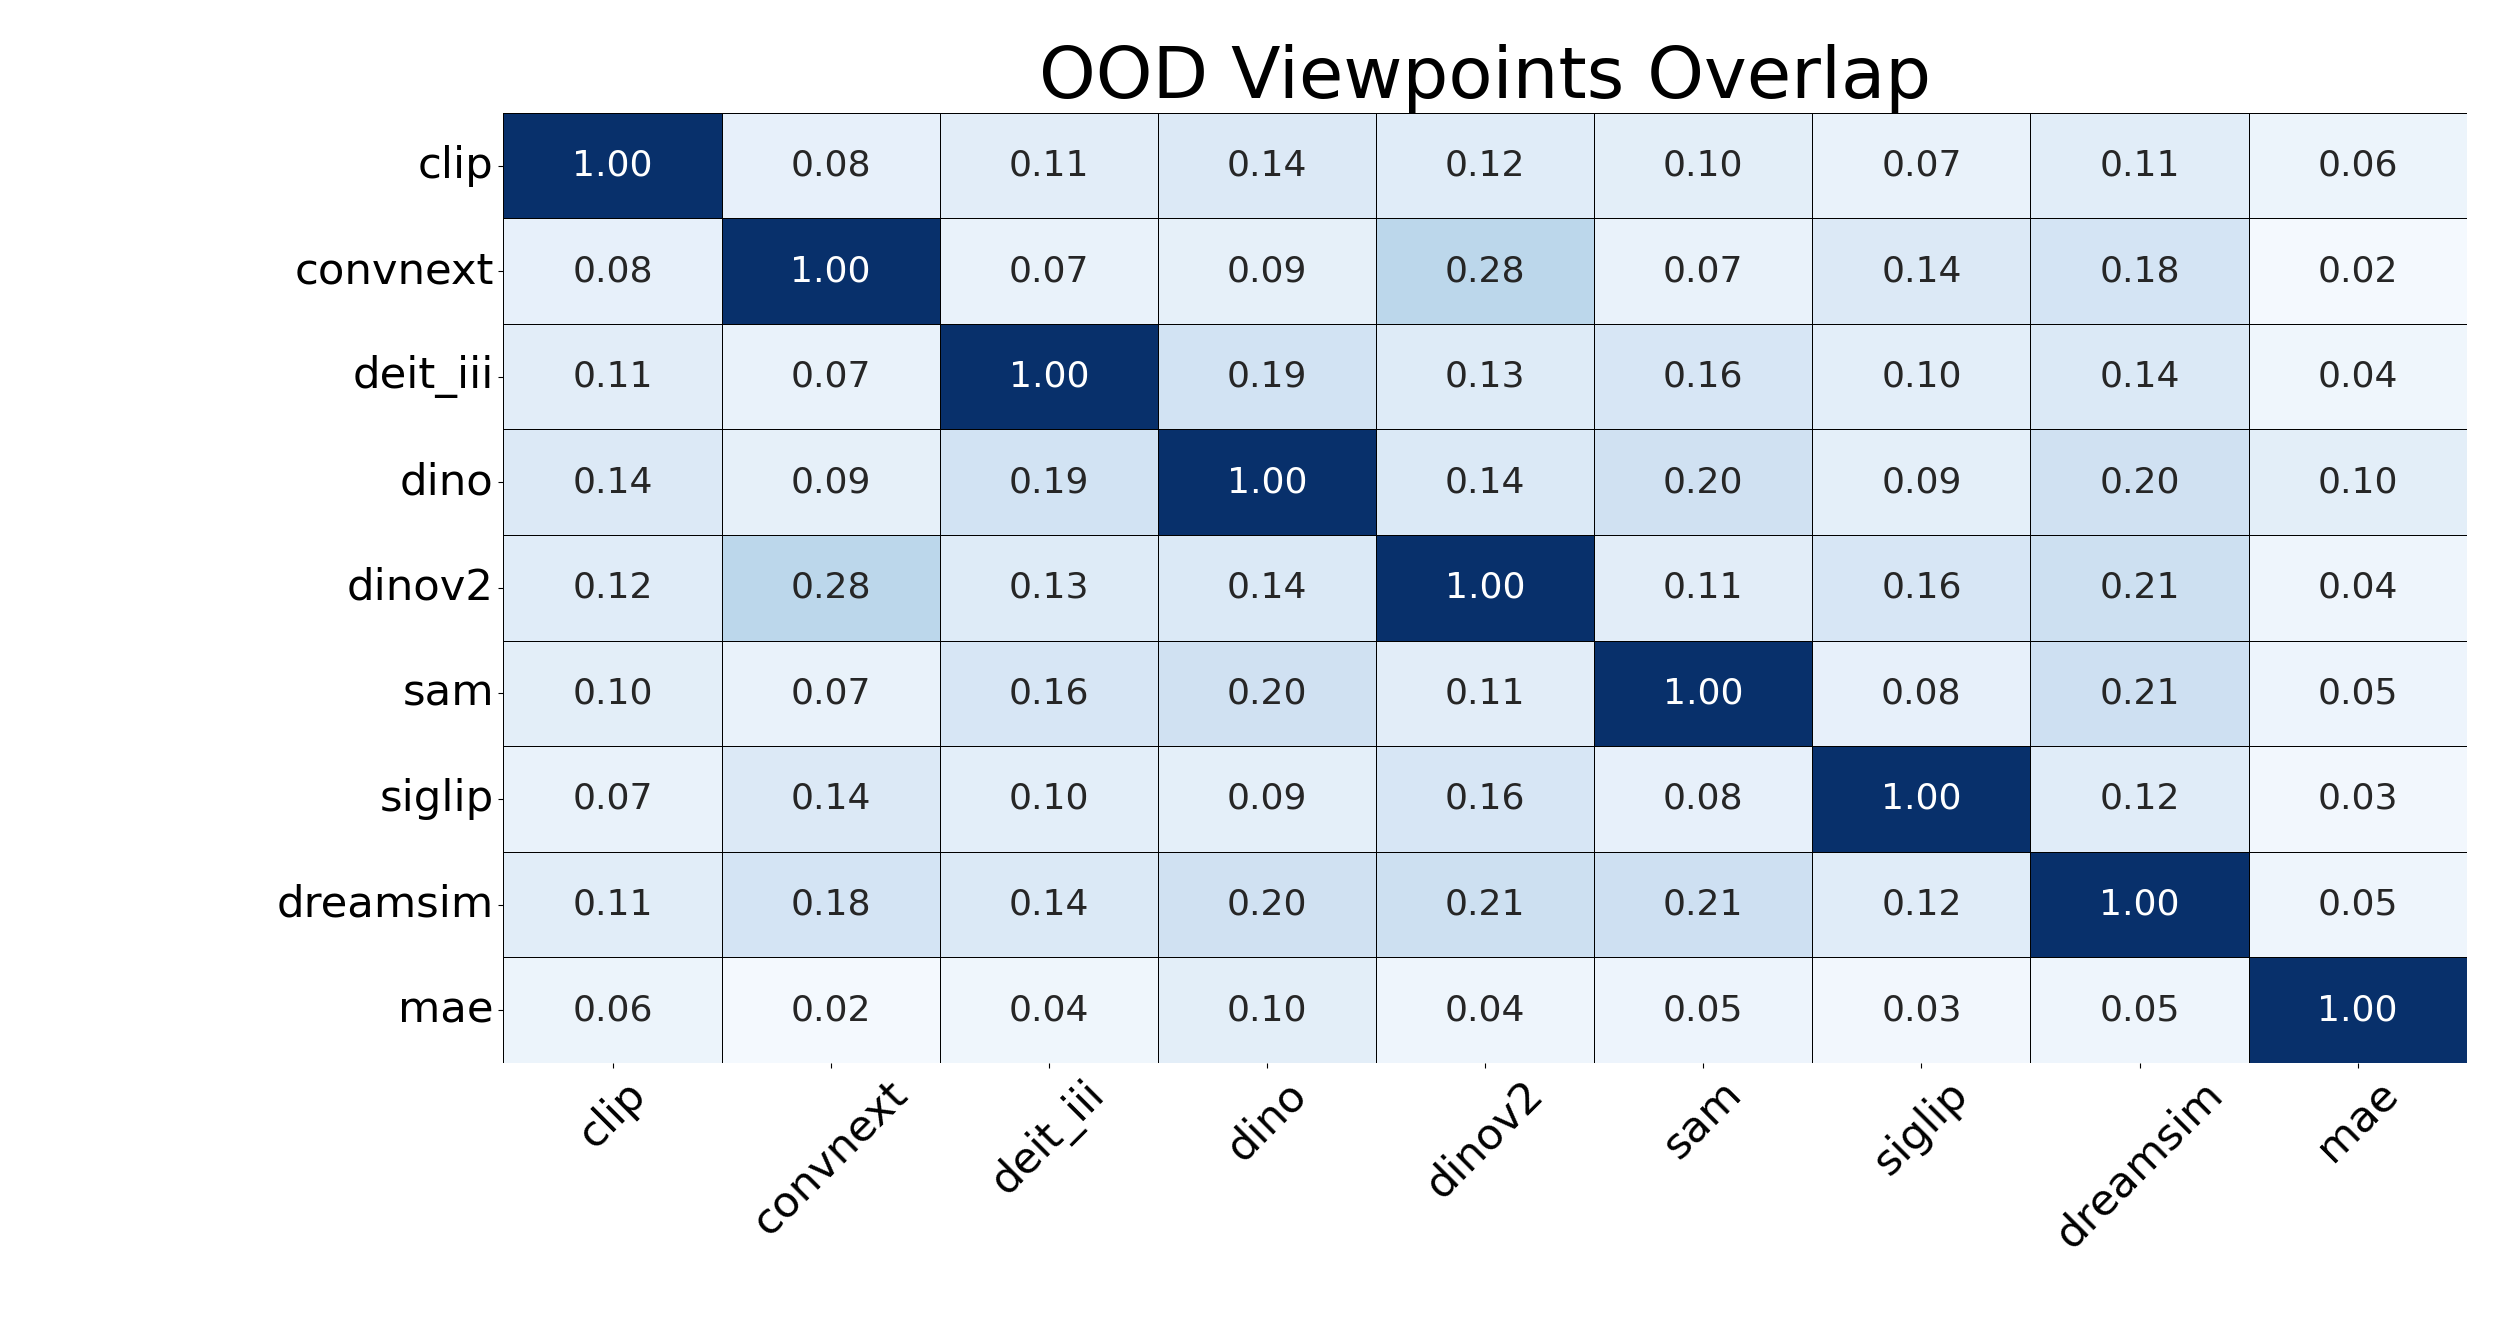}
        % \caption{Caption1 (OOD).}
        \label{fig:subfig_ood}
    \end{subfigure}
\caption{\textbf{Agreement levels on stable, accidental, and OOD viewpoints across nine featurizers, evaluated using Intersection over Union (IoU).} (i) The top-left heatmap shows the mean IoU scores across the nine featurizers for stable, accidental, and OOD viewpoints. (ii) The top-right heatmap displays pairwise IoU scores among the nine featurizers for stable viewpoints, demonstrating strong agreement. (iii) The bottom-left heatmap presents pairwise IoU scores for accidental viewpoints, indicating moderate agreement across featurizers. (iv) The bottom-right heatmap highlights pairwise IoU scores for OOD viewpoints, showing minimal agreement, with many pairs of featurizers exhibiting no overlap (IoU scores under 0.1).}
    \label{fig:merged_figure}
\end{figure*}

\section{Cluster Samples Across Additional Featurizers}

We presents samples from accidental and OOD clusters for the seven featurizers not included in the main paper: DeiT III, SAM, SigLip, ConvNeXT, DINOv2, Dreamsim, and MAE. As shown in Fig.~\ref{fig:combined_figure}. The observed trends are consistent across featurizers. 
For accidental views, specific camera orientations obscure an object’s true 3D structure, effectively reducing its perceived dimensionality by collapsing one axis of depth or perspective.
For OOD views, we observe uncommon orientations, such as objects seen from the back or upside down, as well as instabilities caused by varying lighting conditions. The CO3D dataset, being more complex, introduces additional sources of instability, including occlusions and image blur.

\begin{figure*}[t!]
    \centering
    \includegraphics[width=\linewidth]{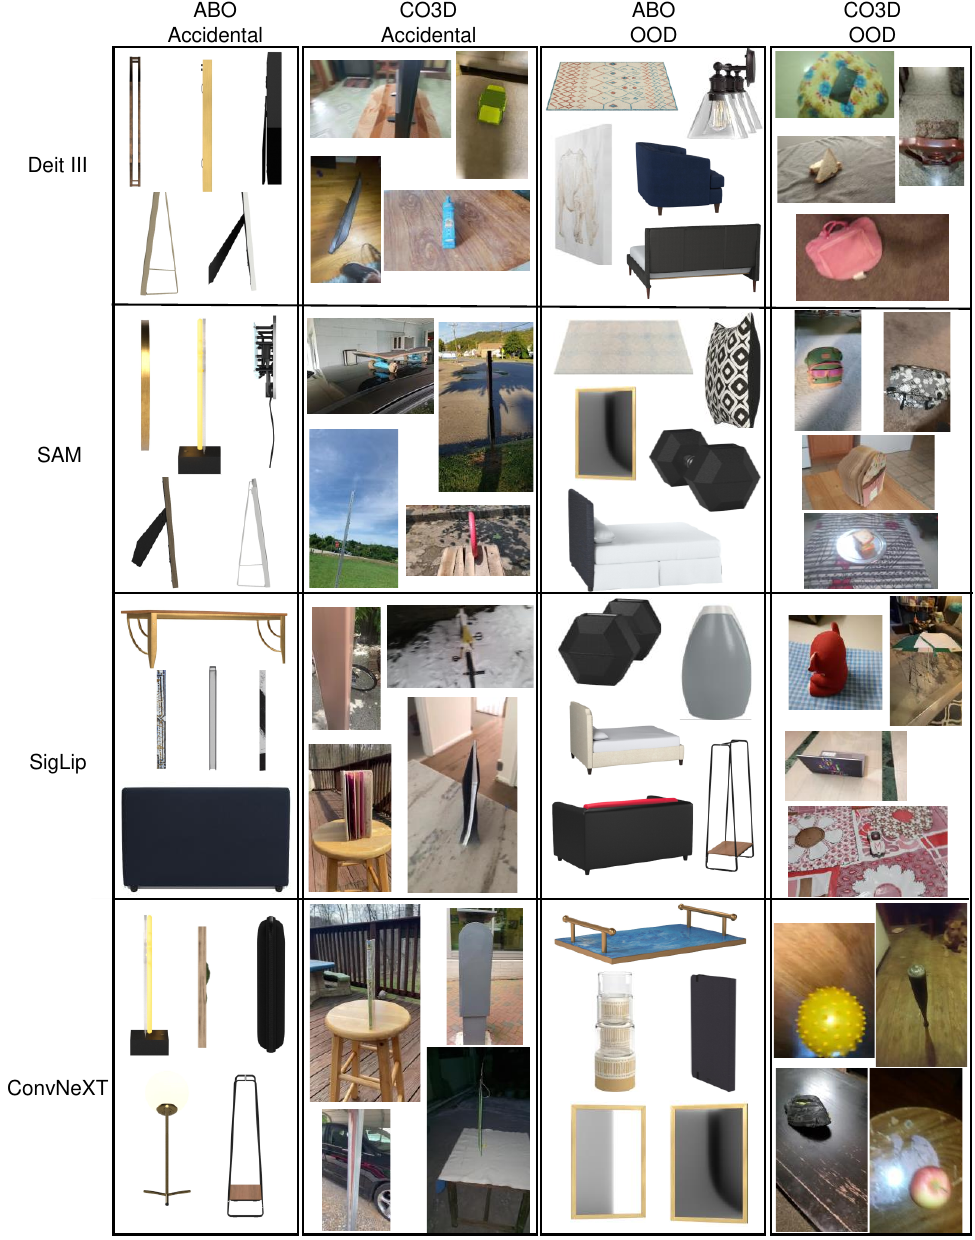}
    \caption*{Figure continues on next page.}
    \label{fig:combined_figure_part1}
\end{figure*}

\begin{figure*}[t!]
    \centering
    \includegraphics[width=\linewidth]{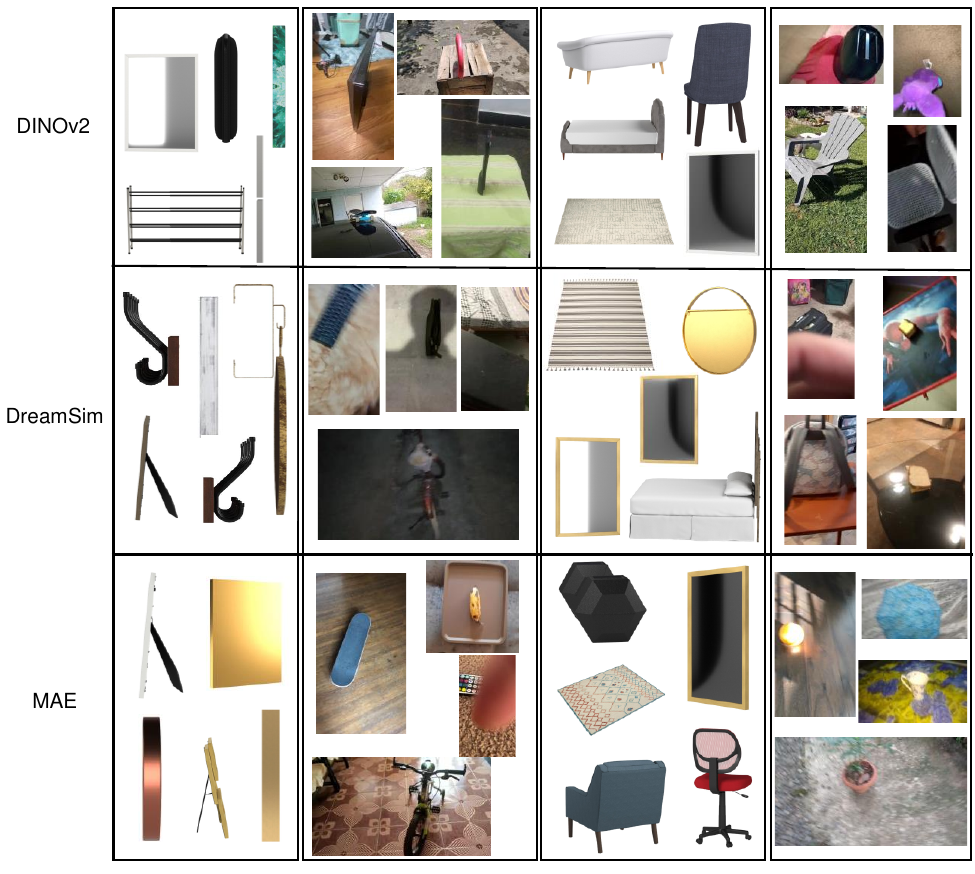}
\caption{\textbf{Examples of accidental and OOD viewpoints using ConvNeXT, DeiT III, DINOv2, Dreamsim, MAE, SAM, and SigLip embeddings across the ABO and CO3D datasets.} Similar to CLIP and DINO discussed in the main paper, accidental views obscure an object's true structure, effectively reducing its perceived dimensionality. OOD views present uncommon orientations, such as objects seen from the back or upside down, and are also affected by sudden lighting changes. The CO3D dataset, being more complex, introduces additional sources of instability, including occlusions and abrupt changes in focus.\mm{Tighten this; make it more professional}}
    \label{fig:combined_figure}
\end{figure*}

\section{Additional Visual Question Answering (VQA) Examples}

To complement the VQA analysis presented in the main paper, we provide additional qualitative examples in Fig.~\ref{fig:supp_llava_qual}. These examples further highlight LLaVA's capabilities in generating descriptive captions across stable, accidental, and OOD viewpoints. As in the main paper, we used LLaVA-1.5~\cite{liu2024improved}, which leverages CLIP as its backbone.
For stable viewpoints, the generated captions remain accurate and closely align with the ground truth (GT) descriptions. However, for accidental and OOD viewpoints, the captions frequently contain inaccuracies, including misinterpretations of objects and hallucinated details that are not present in the image. For instance, the model might describe a black table as "a laptop sitting on a table," despite the absence of a laptop, or misinterpret a light fixture as an umbrella. We hypothesize that this occurs because the pose of the light fixture in the image resembles a pose commonly associated with umbrellas in the training set, leading the model to incorrectly associate the two objects.
In the case of accidental viewpoints, the 3D structure of objects is often collapsed, making it difficult or even impossible to accurately identify the object. This inherent ambiguity in the viewpoint could be acknowledged by the VQA model, which might express uncertainty about the object's identity rather than providing a confident but inaccurate description. Incorporating mechanisms to quantify or communicate uncertainty in such cases could improve the robustness and reliability of VQA models under challenging viewing conditions.

\begin{figure*}[t!]
    \centering
    \includegraphics[width=\linewidth]{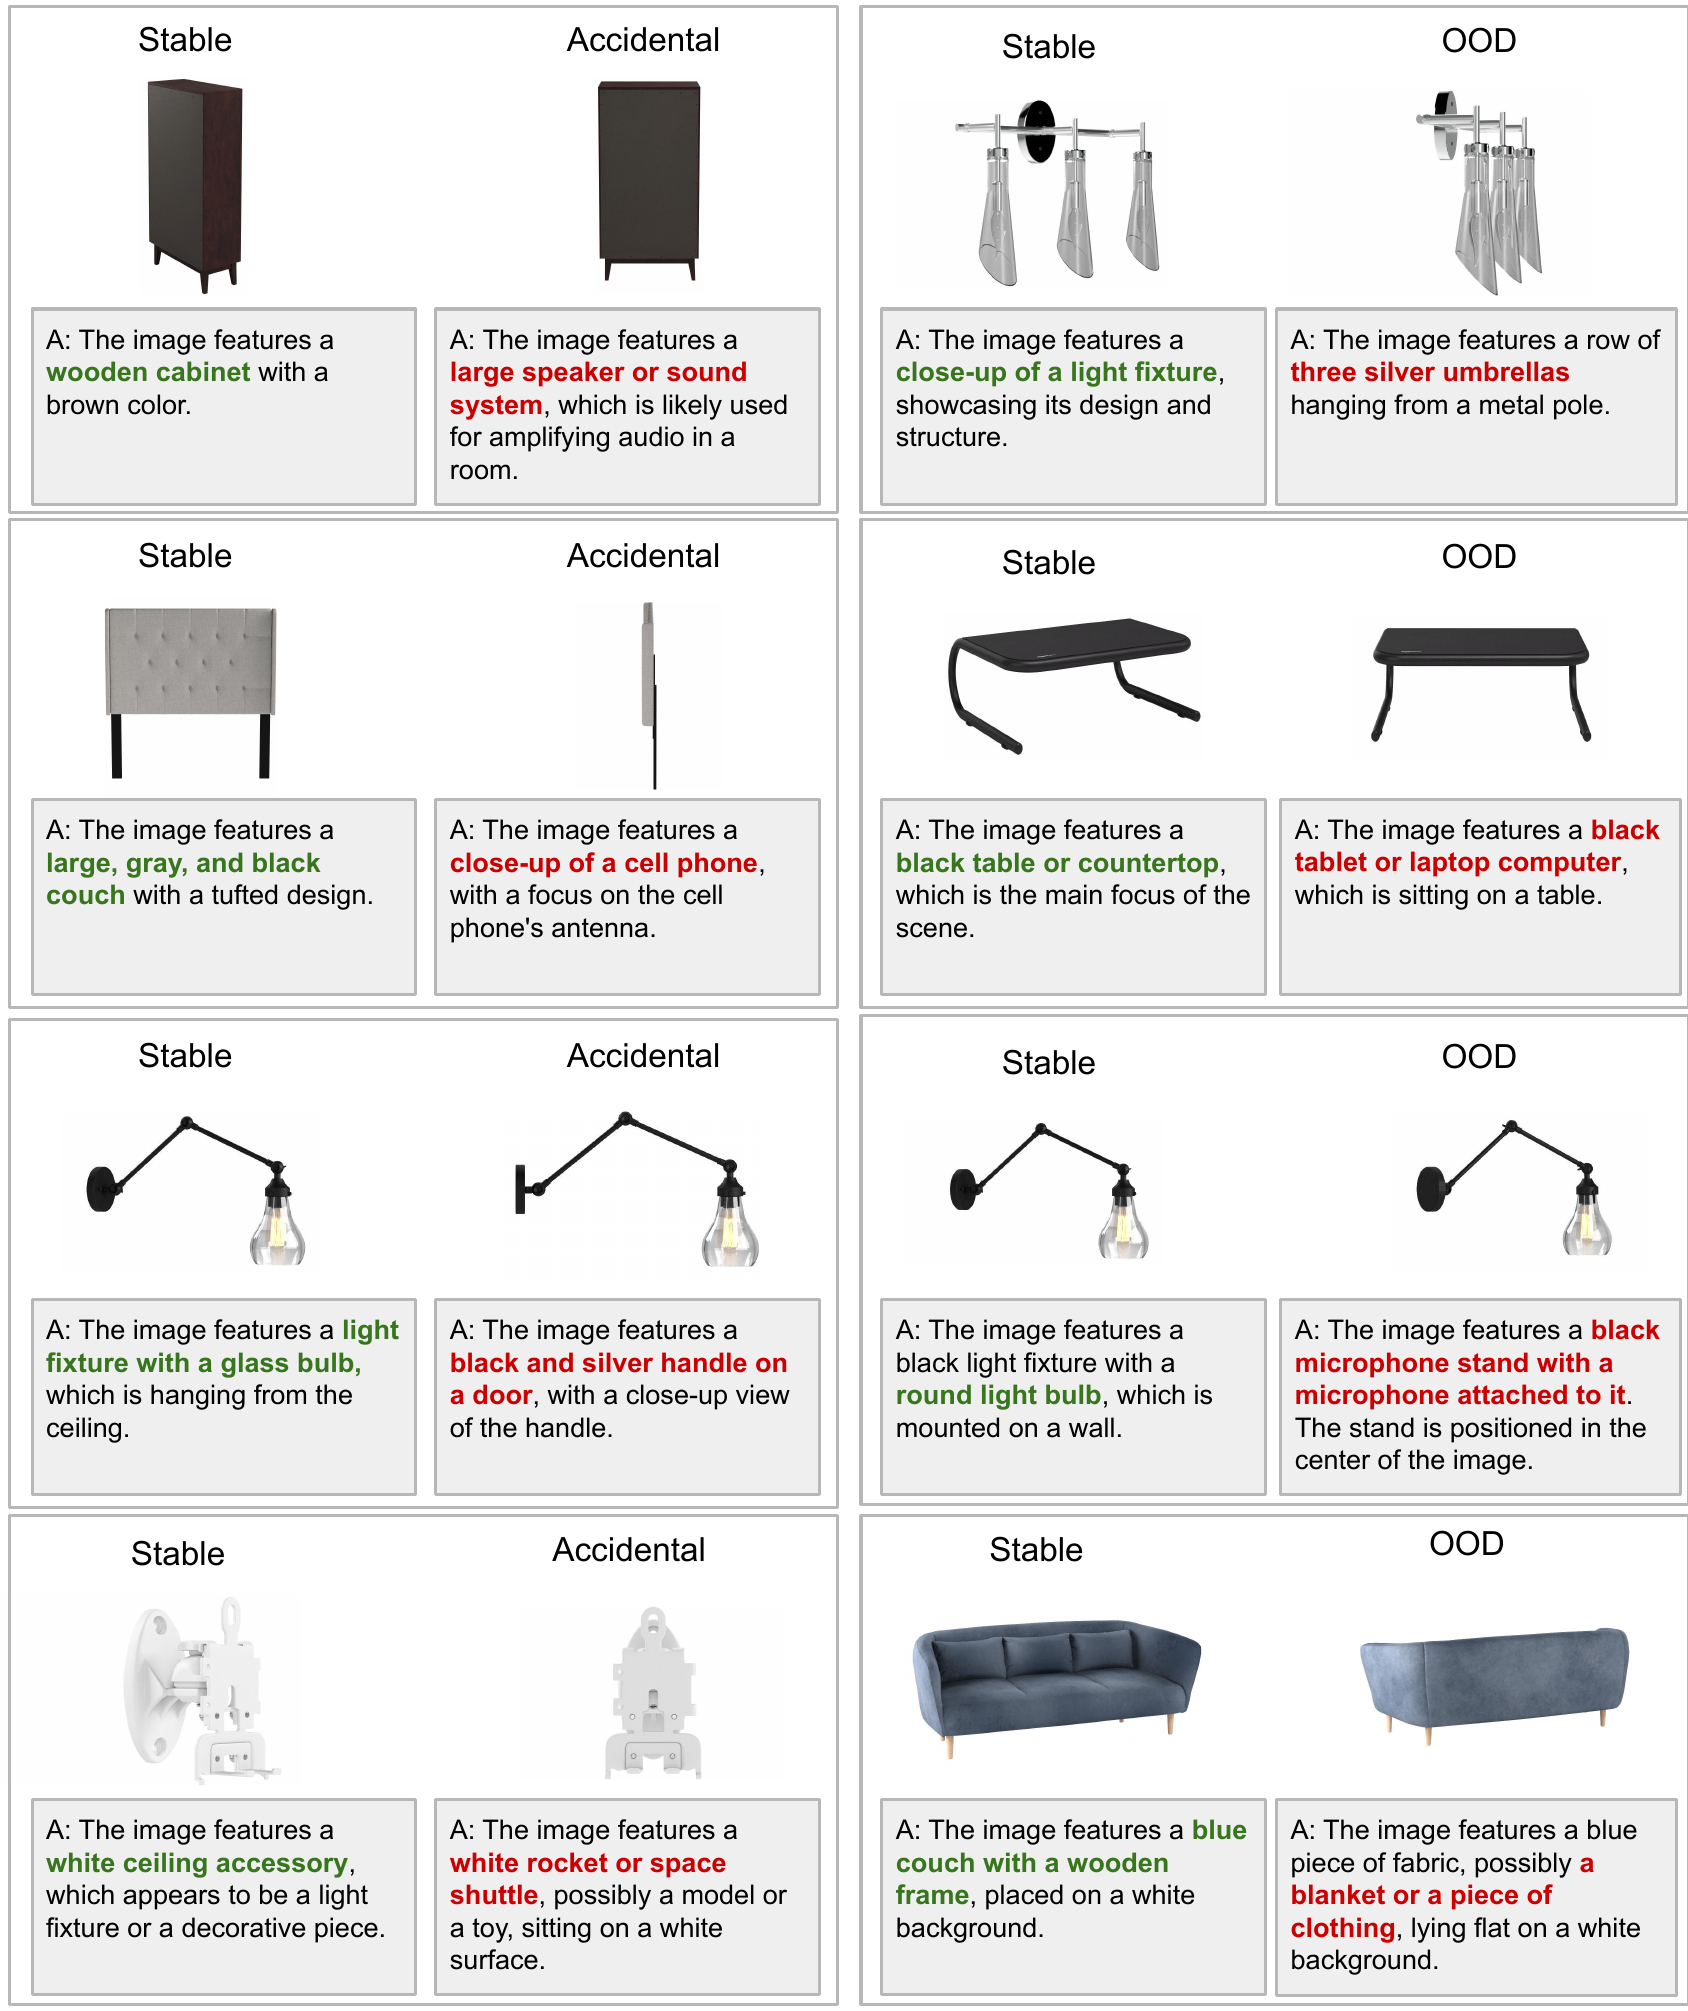}
\caption{\textbf{Examples of generated captions for stable, OOD, and accidental viewpoints using LLaVA-1.5 (CLIP backbone).} Captions for stable viewpoints are accurate, while those for accidental and OOD viewpoints frequently contain inaccuracies, often misinterpreting objects or hallucinating details. For example, a black table might be described as "a laptop sitting on a table," despite no laptop being present.}
    \label{fig:supp_llava_qual}
\end{figure*}

\section{Additional Monocular 3D Reconstruction Results}

To complement the monocular 3D reconstruction analysis presented in the main paper, we provide additional qualitative examples in Fig.~\ref{fig:supp_3dr_samples}. These examples further illustrate the significant impact of viewpoint instability on reconstruction accuracy, using Stable Fast 3D~\cite{boss2024sf3d} with DINOv2~\cite{oquab2023dinov2} as the image featurizer.
For stable viewpoints, the model generates reconstructions with accurate geometry and well-preserved details, aligning closely with the ground truth. However, accidental viewpoints—characterized by insufficient depth cues due to the camera's orientation—result in collapsed or distorted reconstructions. This highlights the challenge of reconstructing 3D shapes when critical geometric information is unavailable.
OOD viewpoints present additional difficulties, as the atypical and rarely seen angles lead the model to misinterpret the object. This results in substantial inaccuracies in the reconstructed shape.

\begin{figure*}[t!]
    \centering
    \includegraphics[width=\linewidth]{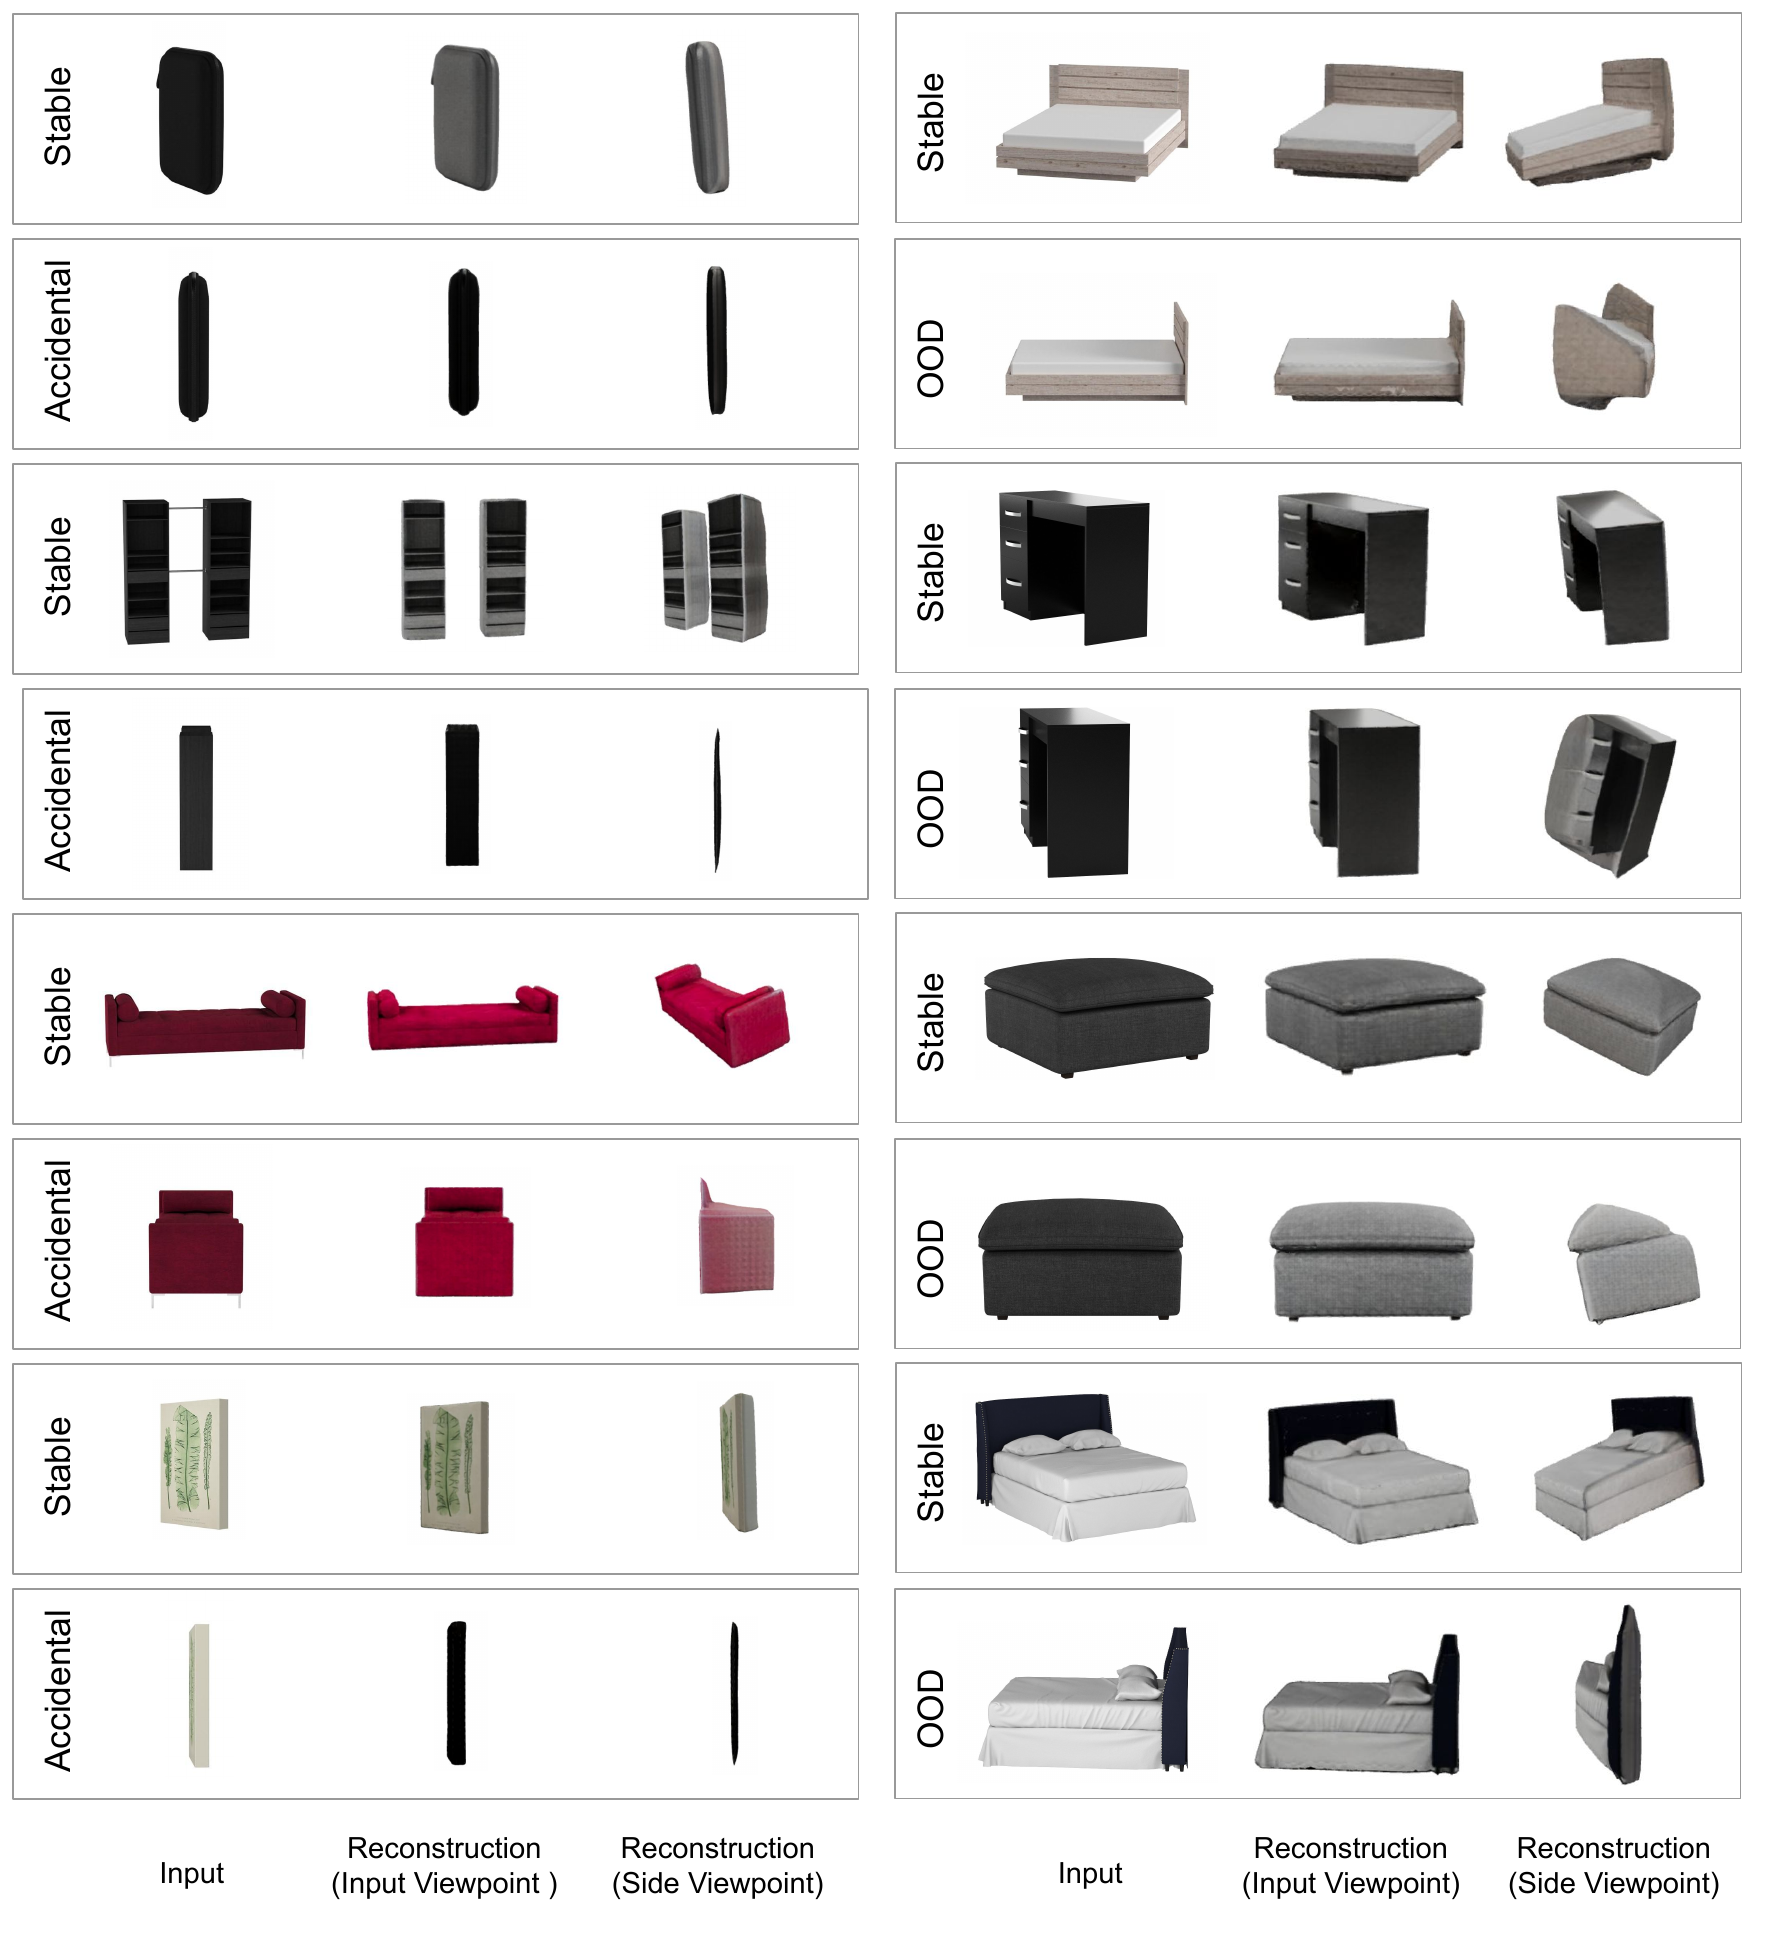}
\caption{\textbf{Additional single-view reconstruction results for stable, accidental, and OOD viewpoints using Stable Fast 3D~\cite{boss2024sf3d} with DINOv2~\cite{oquab2023dinov2} as the image featurizer.} Stable viewpoints yield accurate reconstructions with well-preserved geometry. Accidental viewpoints, lacking sufficient depth cues, result in collapsed or distorted reconstructions. OOD viewpoints, due to atypical angles, often lead to substantial inaccuracies.}
    \label{fig:supp_3dr_samples}
\end{figure*}

%  Main paper ref:
   % Using this approach, we obtained accidFental and OOD clusters for all featurizers, and present random samples from the CLIP and Dino models in Fig.~\ref{fig:cluster_sample_combined}. The CO3D dataset, which includes more complex backgrounds and in-the-wild images, also reveals accidental viewpoints that arise when objects are temporarily occluded. For CO3D OOD views, we often observe objects that appear upside down or temporarily blurry, likely due to changes in focus along the camera’s trajectory. We found similar trends for all other featurizers (see Supplementary).}

 % Main paper ref: 
    % We provide pairwise IoU heatmaps for each label category (stable, acci329 dental, and OOD) across all 9 featurizers in Supplementary.}
